# Supplementary material for: Predator confusion is sufficient to evolve swarming behavior
Source: arXiv:1209.3330 ancillary file (2013-04-03)
Supplement: Supplementary file 1 [file RSI-Predator_Confusion_SI.pdf]

# Supporting Information

Olson et al.

SI Text

## 1 Markov Networks

In a general sense, a Markov Network (MN) implements a probabilistic finite state machine, and as such is a Hidden Markov Model (HMM). MNs act as controllers and decision makers for agents that interact with an environment and agents within the environment. Thus, a MN can be thought of as an *artificial brain* for the agent it controls. Similar to the input and output layer of an artificial neuronal network (ANN), a MN is composed of a set of input nodes (i.e., sensors) and output nodes (i.e., actuators), except that all nodes of a MN are binary, i.e., the nodes can only be in one of two states: 0 or 1. In addition, a MN contains a set of hidden nodes, which act as memory for the MN to store information in.

### How Markov Networks Function

When we embed agents with MNs into an environment and provide it sensorial inputs, these inputs are written into the MN input nodes. Once provided with inputs, we activate MN and all nodes pass information through the MN by updating their states. While input nodes are usually overridden by sensory information from the environment at the beginning of the next brain activation, hidden nodes and output nodes are of particular interest, and their states depend on the particular configuration of the MN. Hidden nodes can be thought of as the memory of the agent or a mechanism to represent an internal state, whereas output nodes determine the action of the agent for that particular point in time. In most cases, the output nodes encode a finite set of actions. For example, two output nodes can be used to steer a tank, according to the output sets in the following table:

| Output A | Output B | Encoded Action |
|----------|----------|----------------|
| 0        | 0        | Stay still     |
| 1        | 1        | Move forward   |
| 0        | 1        | Turn right     |
| 1        | 0        | Turn left      |

Table S2: Example agent action encoding with two output nodes. Each output combination encodes a discrete action taken by the agent.

Arbitrary encodings can be used, but simpler encodings are more conducive to the evolution of effective behavior. In order for agent to be able to react to the environment, the output nodes must somehow connect to the input nodes, and if memory is required for more complex tasks, the output nodes must also depend on the states of hidden nodes. Consequently, hidden nodes might also depend on the input nodes. In a MN, node states are updated by probabilistic logic gates (PLG), also known as a Hidden Markov Gates, which function similar to classic logic gates (e.g., AND, NAND, OR, or XOR). A classic logic gate, e.g. XOR, reads binary states from two input nodes and updates a single output node according to the XOR logic. Alternatively, a classic logic gate can be described with a probability table that maps each possible input to a probability distribution of its outputs. In the case of a XOR gate, there are four possible input sets (00, 01, 10, and 11) and two possible outputs (0 or 1). The following table shows the equivalent probability table of an XOR gate.

While classic logic gates are deterministic, probabilistic logic gates are composed of arbitrary probabilities in their probability table. Therefore, while the output states still depend on the input states, they can also have a degree stochasticity to their output. The above figure illustrates an example PLG, with three binary inputs entering the PLG: 1 and 2 coming from sensory input nodes, while input 3 comes from a hidden node. The PLG is composed of a  $2^2 \times 2^3$  state transition table which encodes the logic for the PLG. Once provided with inputs, the PLG activates and updates the states of hidden node 3 and output node 4. Since the PLG outputs to the same hidden node that it receives input from, it is forming a *recurrent connection*,

| Input A | Input B | p(0) | p(1) |
|---------|---------|------|------|
| 0       | 0       | 1.0  | 0.0  |
| 0       | 1       | 0.0  | 1.0  |
| 1       | 0       | 0.0  | 1.0  |
| 1       | 1       | 1.0  | 0.0  |

Table S3: Probability table for an XOR gate. The input A and input B columns contain the possible states of the input nodes. p(0) and p(1) are the probabilities that the output nodes is a 0 or 1, respectively, given the corresponding input.

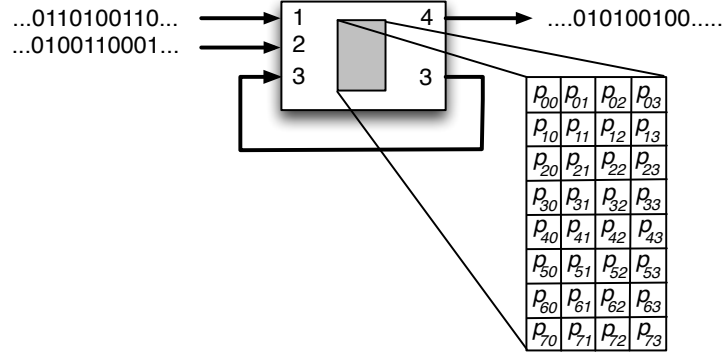

Figure S9: An illustration of a Probabilistic Logic Gate (PLG) with three binary inputs and two binary outputs. The PLG is composed of a  $2^2 \times 2^3$  state transition table which encodes the logic for the PLG.

i.e., memory. The state of output node 4 can encode two possible actions, such as turning left (0) or right (1).

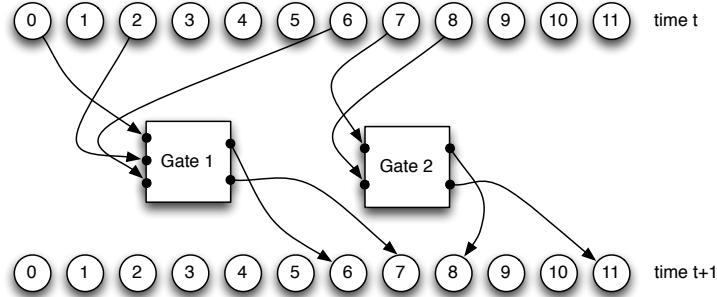

Figure S10: A Markov Network composed of 12 nodes and two Probabilistic Logic Gates (PLGs). Once the nodes at time  $t$  pass binary information into the PLGs, the PLGs activate and update the states of the nodes at time  $t+1$ .

The PLGs we implemented in this model can receive input from a maximum of four nodes, and write into a maximum of four nodes, with a minimum of one input and one output node for each PLG. Any node (input, output, or hidden) in the MN can be used as an input or output for a PLG. MNs are composed of an arbitrary number of PLGs, and the PLGs are what define the internal logic of the MN. Thus, to evolve a MN, mutations change the connections between nodes and PLGs, and modify the probabilistic logic tables that describe each PLG. The figure above demonstrates a MN with 12 nodes connecting to 2 PLGs, and how these two PLGs affect the states of the nodes they write into after one brain activation.

It is possible for two or more PLGs to write into a single node, and each PLG likely has a different

value it wants to place in the common node. This conflict is resolved by using an OR function on the values entering the common node. Thus, whenever one PLG writes a 1 into a node with multiple inputs, that node becomes 1 regardless of the inputs from other PLGs.

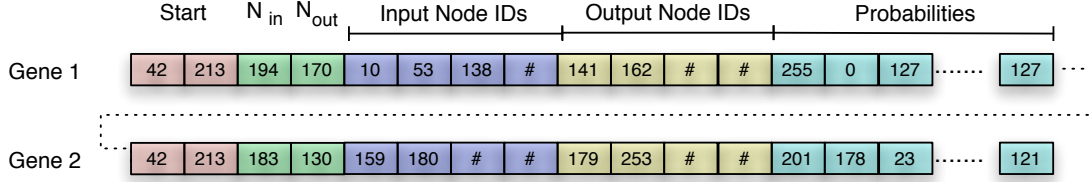

Figure S11: Example circular byte strings encoding two Probabilistic Logic Gates (PLGs), denoted Gene 1 and Gene 2. The sequence (42, 213) represents the beginning of a new PLG (red blocks). The next two bytes encode the number of input and output nodes used by the PLG (green blocks), and the following eight bytes encode which nodes are used as input (blue blocks) and output (yellow blocks). The remaining bytes in the string encode the probabilities of the PLG’s logic table (cyan blocks).

## Genetic Encoding of Markov Networks

We use a circular string of bytes as a genome, which contains all the information to describe a MN. The genome is composed of *genes*, and each gene encodes a single PLG. Therefore, a gene contains the information about which nodes the PLG reads input from, which nodes the PLG writes in to, and the probability table defining the logic of the PLG. The start of a gene is indicated by a *start codon*, which is represented by the sequence (42, 213) in the genome. The specific sequence we chose to represent the start codon is arbitrary; we chose 42 as a tribute to Douglas Adams<sup>1</sup>, and 213 is 255 (the maximum value of a byte) minus 42.

The above figure provides an example genome. After the start codon, the next two numbers describe the number of inputs ( $N_{in}$ ) and outputs ( $N_{out}$ ) used in this gate, where each  $N = \left\lfloor \frac{\text{number}}{255/N_{\max}} \right\rfloor$ . (Here,  $N_{\max} = 4$ .)<sup>2</sup> The following  $N_{\max}$  numbers of the gene specify which nodes the PLG reads from by mapping to a node ID number with the equation:  $\left\lfloor \frac{\text{number} \times \# \text{nodes}}{255} \right\rfloor - 0.5$ , where  $\#$  nodes is the number of nodes in the MN and  $\lfloor \bullet \rfloor$  denotes the nearest integer. Similarly, the next  $N_{\max}$  numbers encode which nodes the PLG writes to with the same equation as  $N_{in}$ . If too many inputs or outputs are specified, the remaining sites in that section of the gene are ignored, designated by the  $\#$  signs.

The following  $2^{N_{in}+N_{out}}$  numbers of the gene expresses the probabilities composing the  $2^{N_{in}} \times 2^{N_{out}}$  logic table. We sequentially fill the logic table row-by-row with numbers from the genome. Once the logic table is filled, we convert the gene numbers into the corresponding probabilities ( $p_{ij}$ ) with the equation:

$$p_{ij} = \frac{1 + \text{number}_{ij}}{\sum_{j=1}^{2^{N_{out}}} (1 + \text{number}_{ij})}$$

Since we use bytes to specify the values in the table, the rows of the probability table are normalized to 1.0. We apply the modulo operator on the number of inputs and outputs as well as the IDs of the nodes used as inputs and outputs in order to keep them within the allowed ranges.

The number of nodes allowed and which nodes are used as inputs and outputs are specified as constants by the user. Combined with these constants, the genome described above unambiguously defines a MN.

<sup>1</sup>This is an inside joke for those who have read Douglas Adams’ book series, “The Hitchhiker’s Guide to the Galaxy.” Therein, the number 42 is “The Answer to the Ultimate Question of Life, the Universe, and Everything,” calculated by an enormous supercomputer over a period of 7.5 million years. When we had to decide what number should be the beginning of the Markov Network codons, the clear answer to us was 42.

<sup>2</sup>We only allow a maximum of 4 inputs and 4 outputs for each Probabilistic Logic Gate (PLG) to encourage evolution to distribute the Markov Network’s (MN) computation across numerous Probabilistic Logic Gates, which unpublished tests have proven to more evolvable in the long run. However, the PLGs in this experiment only make use of 2-3 inputs and outputs at a maximum, so  $N_{\max}$  is never actually reached. Thus, we do not expect the results of the experiment to change at all if we were to increase the maximum. In fact, the fundamental results of the paper are neutral to the substrate that we evolve: Swarming would evolve just as well with Artificial Neural Networks, or any other evolvable “artificial brain” model.

All evolutionary changes such as point mutations, duplication, deletions, or cross over are performed on the genome, and only take effect after the genome is translated into a MN. Thus, the MN can be thought of the phenotype expressed by the genome.

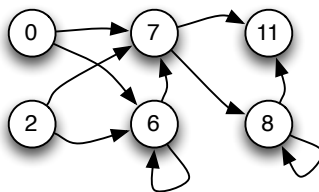

Figure S12: A causal graph of the node connections for a Markov Network (MN). The only nodes displayed are nodes that provide input to or receive output from the Probabilistic Logic Gates of the MN. Arrows between the nodes indicate the flow of binary information between the nodes.

MNs can be visualized in several ways. Since the visualization of the MN in the earlier example is somewhat inconvenient, and the gates are less important than how nodes depend causally on each other, we usually only display a graph similar to the above figure showing the causal relations between the nodes.

## Markov Network FAQ

### Can genes overlap?

Yes, a 42 followed by a 213 defines a start codon. Whenever a start codon is found, the subsequent bytes are used to define a new PLG as well as the remainder of the current PLG. As a consequence of this overlap, a single point mutation can affect multiple genes. This kind of gene overlap is commonly observed in nature.

### Why not use 0 and 255 as start codons?

In prior experiments, we observed that the probabilities in a gene tend to converge on 0 or 255, making the PLGs more deterministic. Therefore, we did not use 0 nor 255 as start codons because an excessive number of genes would end up being encoded.

### Is there directionality in the genes?

We read from the beginning of the sequence to the end in one direction. If a gene extends past the end of the genome byte string, we continue reading at the beginning of the byte string again, i.e., the genome is a circular byte string.

### Why do you OR the output from PLGs that write into the same node instead of preventing gates from writing into the same node?

We do not want to give one gene priority over another gene. If we excluded genes from writing into the same node, we would be required to prioritize which PLG is allowed to write and which one is disallowed. An intuitive method would be to use the order on the genome, such that a PLG which comes earlier in the genome would have priority over other PLGs. We decided against that method, and instead chose to OR the combined outputs. Other output combination methods are possible as well, such XOR, AND, or even thresholds. We experimented with all of these methods and found OR to be the optimal, without having explicit data to support this.

**Since writing into sensors is pointless, why do you allow it?**

On a genetic level, we treat input nodes and output nodes the same way, therefore gates can write into the input nodes of the agent. However, the user decides which nodes are used as inputs or outputs. When we translate a genome into a MN, we don't explicitly know which nodes are inputs and outputs, therefore we allow gates to write into nodes that are designated as inputs. After the brain is activated, sensorial inputs from the environment override anything the gates might have written into them anyway.

**Why do you allow gates to read from actuator?**

Human brains can sense what its muscles are doing and what angle its joints are at, therefore we see no reason to disallow a MN from doing this as well.

## Genetic algorithm and experiment settings

| GA Parameter           | Value                 |
|------------------------|-----------------------|
| Selection              | Fitness proportionate |
| Population size        | 100                   |
| Per-gene mutation rate | 1%                    |
| Gene duplication rate  | 5%                    |
| Gene deletion rate     | 2%                    |
| Crossover              | None                  |
| Generations            | 1,200                 |
| Replicates             | 180                   |

Table S1: Genetic algorithm and experiment settings

## Effects of seeding with pre-evolved predators

We ran a separate set of experiments seeding the predator population with randomly-generated MNs to verify that seeding with a pre-evolved predator had negligible impact on the outcome of the experiment. Figure S1 shows that regardless of how the predator population is seeded, swarming only evolves with the predator confusion mechanism active. Thus seeding the predator population with a pre-evolved predator that exhibits rudimentary prey tracking behavior only serves to speed up the coevolutionary process.

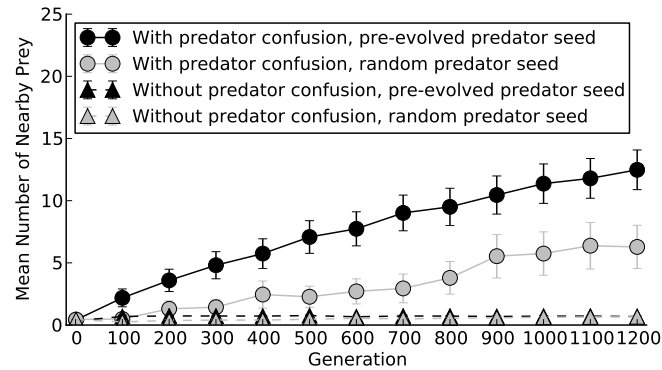

Figure S1: Mean swarm density over all replicates over evolutionary time, measured by the mean number of prey within 30 virtual meters of each other over a lifespan of 2,000 simulation time steps. Prey in swarms with predator confusion (black and grey circles with a full line) evolve to maintain significantly higher swarm density than prey in the swarms without predator confusion (black and grey triangles with a dashed line), regardless of how the predator population is seeded. Error bars indicate two standard errors over 100 replicates.

### Effects of predator handling time on the evolution of swarming behavior

We ran a another set of predator confusion experiments to determine if a predator handling time lower than 10 had a significant impact on the outcome of the experiment. Figure S2 provides evidence that cohesive swarming behavior evolves in prey when they are hunted by a predator with predator confusion regardless of the handling time, except when there is no handling time at all. Assigning the predator a handling time of 0 is unrealistic, however, because that allows the predator to make an unlimited number of capture attempts when it gets close to prey. Therefore, we used a default value of 10 in our experiments as an reasonable handling time.

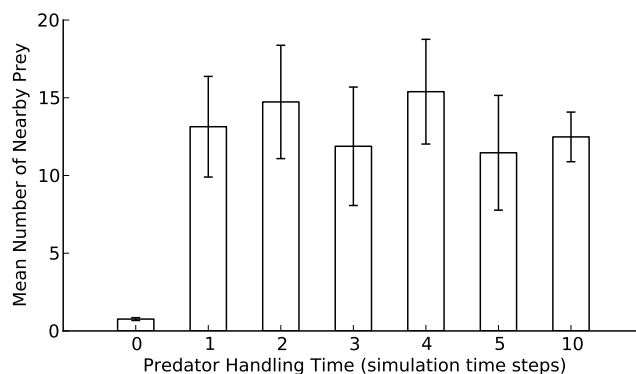

Figure S2: Mean swarm density for each handling time over all replicates at generation 1,200, measured by the mean number of prey within 30 virtual meters of each other over a lifespan of 2,000 simulation time steps. Prey hunted by predators with predator confusion evolve cohesive swarming behavior regardless of the handling time, as long as there is a delay of at least 1 simulation time step between capture attempts. Error bars indicate two standard errors over 100 replicates.

### Costs of grouping for prey

Although predator confusion provides an advantage to grouping prey in this model, there are costs of grouping as well. Figures S3 and S4 demonstrate that as prey hunted by a predator with predator confusion evolve increasingly cohesive swarming behavior, they also experience significantly more attacks from the predator than the prey that evolved dispersive behavior without predator confusion. This is likely because the prey are all centralized in a single location, so the predator does not have to spend any time searching for prey to attack. For grouping behavior to evolve, the benefits of grouping (in this case, reduced predator attack efficiency due to predator confusion) must outweigh the cost of grouping.

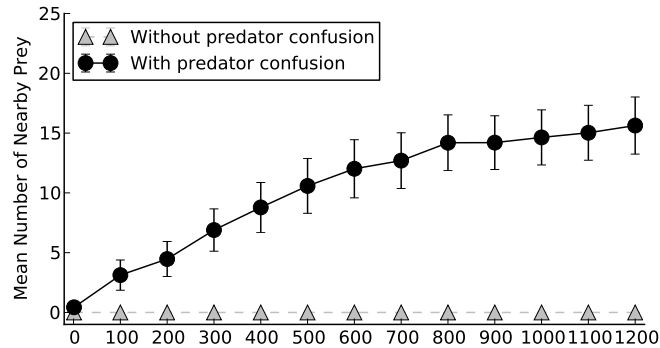

Figure S3: Mean swarm density over all replicates over evolutionary time, measured by the mean number of prey within 30 virtual meters of each other over a lifespan of 2,000 simulation time steps. Prey hunted by a predator with predator confusion (black circles with a full line) evolved to maintain significantly higher swarm density than prey in the swarms hunted by a predator without predator confusion (grey triangles with a dashed line). Error bars indicate two standard errors over 100 replicates.

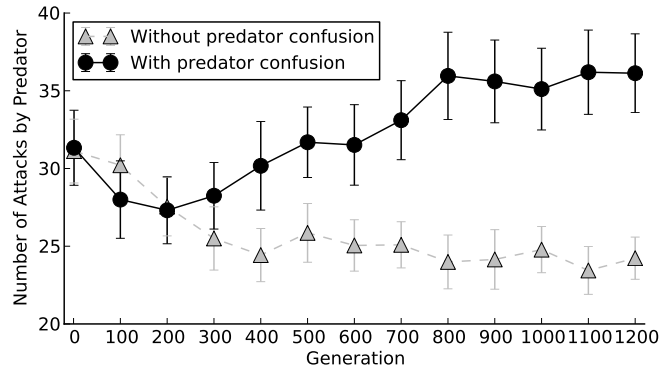

Figure S4: Mean number of attacks attempted on the swarm by the predator over evolutionary time. As the prey hunted by a predator with predator confusion (black circles with a full line) evolved increasingly cohesive swarming behavior, they also experienced significantly more attacks from the predator than prey in the swarms hunted by a predator without predator confusion (grey triangles with a dashed line). Error bars indicate two standard errors over 100 replicates.

### Predator attack efficiency as a function of nearby and visible prey

Attack efficiency curves plot the percentage chance a predator has of making a successful attack on a prey when the given number of prey are near the target prey and visible to the predator. Figure S5 illustrates some of the attack efficiency curves we explored, including the  $\frac{1}{N}$  curve used in the main experiment.

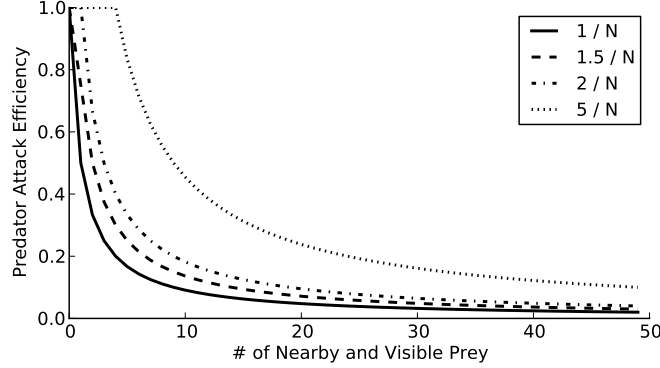

Figure S5: Some of the attack efficiency curves explored for this project. Each function defines the percentage chance a predator has of successfully capturing a prey given  $N$ , the number of prey that are near the target prey and visible to the predator. For example, for the  $\frac{5}{N}$  equation, the predator has a 50% chance of successfully capturing the prey if there are 10 prey near the target prey and visible to the predator.

We found that the evolution of swarming behavior is sensitive to the predator's attack efficiency curve caused by predator confusion. Using the attack efficiency curves in Figure S5, we ran another set of experiments to determine whether swarming behavior evolves with each attack efficiency curve. Figure S6 shows that decreasing the effectiveness of predator confusion can result in prey no longer evolving swarming behavior (e.g., with the  $\frac{5}{N}$  attack efficiency curve). Thus it is possible for the costs of grouping (Figure S4) to outweigh the benefits of grouping from predator confusion.

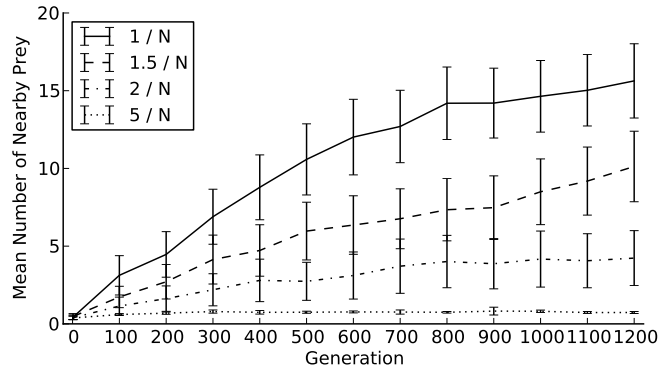

Figure S6: Mean swarm density over all replicates over evolutionary time, measured by the mean number of prey within 30 virtual meters of each other over a lifespan of 2,000 simulation time steps. Prey evolved with attack efficiency curves providing a strong predator confusion effect, e.g.  $\frac{1}{N}$  (full line) and  $\frac{1.5}{N}$  (dashed line), evolve cohesive swarming behavior, whereas prey evolved with attack efficiency curves providing a weak predator confusion effect, e.g.  $\frac{2}{N}$  (dashed and dotted line) and  $\frac{5}{N}$  (dotted line), evolved loose swarms or completely dispersive behavior. Error bars indicate two standard errors over 100 replicates.

We investigated the impact of capping the predator’s attack success rate at a minimum of 20%, making it impossible for the predator confusion effect to make the predator entirely ineffective. As Figure S7 shows, even with a minimum threshold of a 20% success rate, the prey hunted by predators with predator confusion still evolve cohesive swarming behavior.

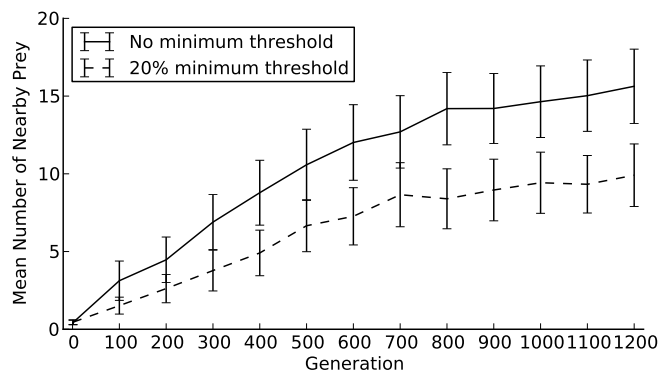

Figure S7: Mean swarm density over all replicates over evolutionary time, measured by the mean number of prey within 30 virtual meters of each other over a lifespan of 2,000 simulation time steps. Prey hunted by predators with predator confusion evolve cohesive swarming behavior, regardless of whether the attack efficiency curve has a minimum threshold of a 20% success rate (dashed line) or no minimum threshold at all (solid line). Error bars indicate two standard errors over 100 replicates.

### Effects of predator view angle on predator capture rate

Reducing the predator's view angle increases its capture rate because it is less confused by swarming prey (Figure S8). Interestingly, there appears to be a predator view angle around  $30^\circ$  where even though the predator confusion effect is entirely cancelled (Figure 5 - main text), having such a small retina reduces the predator's capture rate.

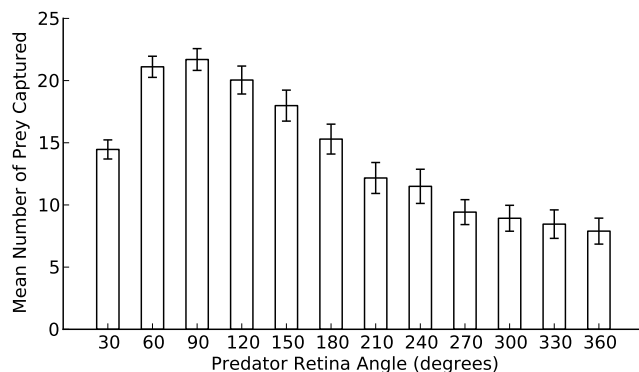

Figure S8: Mean number of prey captured for each predator view angle over all replicates at generation 1,200. Predators with a higher view angle capture significantly fewer prey due to the prey swarming and exploiting the predator confusion effect. Error bars indicate two standard errors over 100 replicates.

### Effects of predator handling time on functional response

Additionally, we measured the impact of handling time on predator functional response in the predator confusion experiments. Figure S9 shows the expected trend: as the handling time is increased, the predator reaches the plateau at which it can no longer consume any more prey regardless of prey density earlier and at a significantly lower consumption rate. Thus handling time plays an important role in the ecology of the evolutionary system.

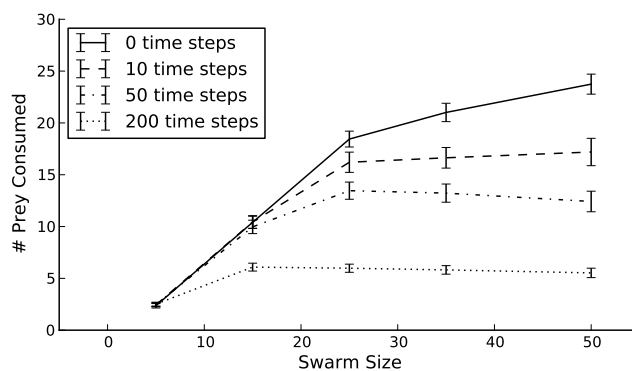

Figure S9: Functional response curves of cohesive swarms hunted by a predator with predator confusion with handling times of 0 (solid line), 10 (dashed line), 50 (dashed and dotted line), and 200 (dotted line). Increasing the predator's handling time decreases the predator's prey consumption rate. Error bars indicate two standard errors over 100 replicates.

### Why does swarm density appear to still be increasing at generation 1,200?

Plotting the runs individually clarifies this situation. Some populations evolve swarming behavior early on in evolutionary time (Figure S10A), while other populations take longer to discover the proper sequence of mutations to evolve swarming behavior (Figure S10B). Since the plot we show in the paper is the mean swarm density at each generation, the gradual rise in the mean over time is due to an increasing number of populations evolving swarming behavior. As we stated in the paper, even at generation 1,200, only 70% of the populations had evolved swarming. Looking at the runs where swarming evolved early on, the maximum achievable swarm density appears to be 30-35, which is the circular swarm behavior shown in the paper and SI videos. Thus, if we kept running the simulation yet more generations, the mean would only continue to rise up to 25-30 swarm density as the remainder of the populations finally evolved swarming behavior, then it would plateau there.

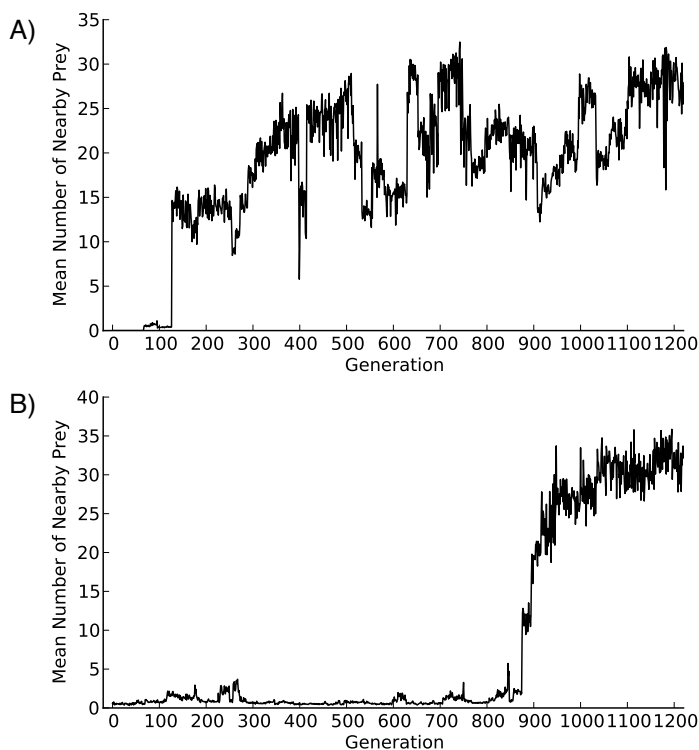

Figure S10: Swarm density over two individual replicates over evolutionary time, measured by the mean number of prey within 30 virtual meters of each other over a lifespan of 2,000 simulation time steps. These two graphs show how swarming behavior evolves at different generations, which can make the mean swarm density over all replicates look like it is still increasing at generation 1,200.

## **Swarm Visualizations**

We construct the visualizations of the swarm by placing the MNs of a single predator and prey of interest in a fitness evaluation simulation (see Methods section for detail on fitness evaluation simulations). For every time step in the simulation, we record the location of each living predator and prey and pipe the data to a separate Processing program that creates a video of the simulation. The code for the simulation and visualization software are available on Github at: <https://github.com/adamilab/eos>.

## **Data Analysis and Availability**

We used IPython Notebook for the statistical analyses and graph generation for this publication, which is available online along with the data from these experiments at <https://github.com/adamilab/eos-data>.

## 2 SI Videos

These videos show the lifetime of the highest fitness predator and prey (2,000 simulation time steps) at the end of 1,200 generation of evolution, from 5 selected independent evolution experiments. Prey are randomly placed within the  $512 \times 512$  arena. The swarm "phenotype" (the particular swarming behavior) does not depend on the initial condition, but the number of swarms that form, whether they will merge or separate, does depend on the initial placement of agents. For the purposes of visualization, 100 prey were cloned from a single genotype, as opposed to the 50 prey used in the fitness evaluation during the actual evolution experiment.

**SI Video 1.** Typical prey behavior when predators are not confused by multiple prey in their visual field. The prey spread out as much as possible while moving around randomly.

**SI Video 2.** Example swarm behavior when predators are confused by multiple prey in their visual field. The prey form multiple cohesive, circular swarms to maximize the confusion effect for the predator.

**SI Video 3.** Example swarm behavior when predators are confused by multiple prey in their visual field. The prey aggregate into single swarm that changes shape multiple times throughout the simulation.

**SI Video 4.** Example swarm behavior when predators are confused by multiple prey in their visual field. The prey form a dispersed swarm that splits apart into two swarms at one point, then merges back together into a single swarm.

**SI Video 5.** Example swarm behavior when predators are confused by multiple prey in their visual field. The prey form a massive, chaotic swarm in the center of the simulation space.
